# Supplementary material for: Enhancing Large Language Models for Hardware Verification: A Novel SystemVerilog Assertion Dataset
Source: arXiv:2503.08923 source file (2025-03-11)
Supplement: Supplementary file 1 [file appendix.tex]

%%%%%%%%%%%%%%%%%%%%%%NO APPENDIX%%%%%%%%%%%%%%%%%%%%%%%%%%%%%%%%%%

% % Reset tocdepth for sections you want to appear
\addtocontents{toc}{\setcounter{tocdepth}{2}} % Include sections starting from this point
% \tableofcontents

% Adjustments for the Table of Contents format
          % Section titles in bold
     % Subsection titles in normal font
             % Dot after section number
          % Dot after subsection number
      % Bold page number for sections

% Customize section numbering for the appendix

% Table of Contents for the appendix
\newpage
\tableofcontents

\section{Appendix}
\label{sec:app}

\subsection{Dataset Examples}
\label{synthetic_examples}

Figure~\ref{listings} presents synthetic SystemVerilog code snippets and their formal assertions from our dataset. The left column shows representative code blocks with conditional and case-based logic. The top-left snippet is from the “if-else” dataset, where the assertion checks that when \texttt{!cfg\_7} is true and \texttt{hw\_13 \&\& reg\_14 || core\_17} holds, \texttt{chip\_9} must equal \texttt{fsm\_18}. This ensures correct signal assignment following the logic during simulation or formal verification.

The middle-left snippet, from the “case” dataset, assigns \texttt{chip\_12} to \texttt{tx\_10} if \texttt{flag\_register\_18} equals \texttt{5'b10011}. The corresponding assertion ensures that this assignment occurs correctly. The bottom-left snippet showcases a case statement where if \texttt{flag\_register\_18} is \texttt{7'h26} and the compound condition (\texttt{rx\_6 || rx\_1 || hw\_7}) holds, \texttt{cfg\_20} and \texttt{reg\_3} are assigned the expected values, formalized by an assertion.

% Explain the flowchart
\begin{figure}[h]
    \begin{subfigure}[c]{0.47\textwidth}
        %\hspace{-0.8cm}
        \input{Snippets/listing_ifelse}
    \end{subfigure}
    \hspace{1mm}
    \begin{subfigure}[c]{0.06\textwidth}
        % \hspace{5mm}
        \includegraphics[width=\textwidth]{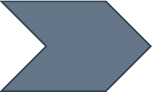}
    \end{subfigure}
    \hfill
    \begin{subfigure}[c]{0.47\textwidth}
        \input{Snippets/listing_ifelse_assertions}
    \end{subfigure}
    %%%%%%%%%%%%%%%%%%%%%%%%%%%%%%%%%%%%second row
    \begin{subfigure}[c]{0.47\textwidth}
        \input{Snippets/listing_case}
    \end{subfigure}
    \hspace{1mm}
    \begin{subfigure}[c]{0.06\textwidth}
        % \hspace{5mm}
        \includegraphics[width=\textwidth]{Figures/Chevron.pdf}
    \end{subfigure}
    \hfill
    \begin{subfigure}[c]{0.47\textwidth}
        \input{Snippets/listing_case_assertions}
    \end{subfigure}
    %%%%%%%%%%%%%%%%%%%%%%%%%%%%%%%%%%%%3 row
    \begin{subfigure}[c]{0.47\textwidth}
        \input{Snippets/listing_caseif}
    \end{subfigure}
    \hspace{1mm}
    \begin{subfigure}[c]{0.06\textwidth}
        % \hspace{5mm}
        \includegraphics[width=\textwidth]{Figures/Chevron.pdf}
    \end{subfigure}
    \hfill
    \begin{subfigure}[c]{0.47\textwidth}
        \input{Snippets/listing_caseif_assertions}
    \end{subfigure}
    \caption{Examples of code blocks (left) and their corresponding assertions (right) in our dataset.} % CLOCKWISE FROM TOP 
    \label{listings}
\end{figure}

\subsection{Fine-Tuning}
\label{sec:fine_tune}
%For fine-tuning, we use the following hyper-parameters outlined in Table \ref{tab:param} and explained below:

% To effectively utilize LLMs on the task of assertion generation, it is crucial to transform the raw dataset into a format that aligns with the input structure expected by the pre-trained model. This step involves creating prompt templates incorporating previously generated HDL code and the relevant assertions into the system prompt expected by the pre-trained model.

We utilized the hyperparameters detailed in Table \ref{tab:param}, leveraging the Low-Rank Adapter (LoRA) technique with a rank and alpha of 256 to optimize the model for hardware verification tasks with minimal computational overhead. This configuration allowed for efficient low-rank updates, preserving the core model's behavior while integrating task-specific adjustments. A maximum sequence length of 4096 tokens was employed to accommodate longer logic and condition sequences in assertion generation, with training constrained to 3 epochs to avoid overfitting. \input{Tables/hyperparam} We selected a batch size of 64 and a learning rate of $1.00e^{-04}$ for computational efficiency and stable convergence, with Bf16 precision enhancing training speed without compromising accuracy. By targeting the \texttt{Query}, \texttt{Key}, \texttt{Value}, \texttt{Output}, and \texttt{Gate} layers, we effectively adapted the model while updating only 4-6\% of its parameters, thus optimizing performance while controlling computational costs.

% We employed a set of hyperparameters, as outlined in Table \ref{tab:param}.

% The Low-Rank Adapter (LoRA) technique with a rank of 256 and a matching LoRA alpha of 256 optimizes the model’s adaptation to hardware verification tasks while requiring minimal computational resources. This setup ensured low-rank updates scaled effectively, preserving original model dynamics while introducing task-specific modifications. A maximum sequence length of 4096 tokens was used to handle the longer logic and condition sequences in assertion generation, with training limited to 3 epochs to prevent overfitting. A batch size of 64 and a learning rate of $1.00e^{-04}$ were chosen for computational efficiency and convergence stability, and training used Bf16 precision to accelerate the process while maintaining accuracy. We targeted the \texttt{Query}, \texttt{Key}, \texttt{Value}, \texttt{Output}, and \texttt{Gate} layers, optimizing adaptation by training only 4-6\% of the model’s parameters while managing computational costs.

\subsection{Examples comparing Fine-tuned model to Base model}
\label{fine_base_assert_examples}
\subsubsection{OpenTitan assertion examples}
\label{open_assert_examples}
\begin{tcolorbox}[colback=white, colframe=black, boxrule=0.2mm, sharp corners, title=DeepSeek Coder input prompt, coltitle=black, colbacktitle=white]
\#\#\# Instruction: Generate a list of synchronous SystemVerilog assertions executing at posedge clk\_i from the following code: 
\lstset{style=mystyle2}
\begin{lstlisting}[language=Verilog]
    if (!rst_ni) begin
      edn_req_hold_q <= '0;
    end else begin
      edn_req_hold_q <= edn_req_hold_d;
    end
\end{lstlisting}
 \#\#\# Response: 
\end{tcolorbox}

% \lstset{style=mystyle}
% \begin{lstlisting}[language=Verilog]
% The given code is a synchronous systemverilog code for a flip-flop. It is a simple register that holds its value on the rising edge of the clock signal `clk_i`. The reset signal `rst_ni` is used to clear the register.

% The synchronous systemverilog assertion executing at posedge clk_i would be:

% ```systemverilog
% assert property (
%   @(posedge clk_i) disable iff (~rst_ni)
%     (edn_req_hold_q == $past(edn_req_hold_d, 1))
% );
% ```

% This assertion checks that the value of `edn_req_hold_q` is equal to the value of `edn_req_hold_d` at the previous clock cycle. The `$past` function is used to access the value of `edn_req_hold_d` from the previous cycle. The `disable iff (~rst_ni)` part ensures that the assertion is not checked when `rst_ni` is low.
% \end{lstlisting}

\begin{tcolorbox}[colback=white, colframe=black, boxrule=0.2mm, sharp corners, title= DeepSeek Coder base model response, coltitle=black, colbacktitle=white]
The given code is a synchronous systemverilog code for a flip-flop. It is a simple register that holds its value on the rising edge of the clock signal `clk\_i'. The reset signal `rst\_ni' is used to clear the register.

The synchronous systemverilog assertion executing at posedge clk\_i would be:

% \vspace{2mm}\textbf{SystemVerilog:}
\lstset{style=mystyle2}
\begin{lstlisting}[language=Verilog]
assert property (
  @(posedge clk_i) disable iff (~rst_ni)
    (edn_req_hold_q == $past(edn_req_hold_d, 1))
);
\end{lstlisting}

This assertion checks that the value of `edn\_req\_hold\_q' is equal to the value of `edn\_req\_hold\_d' at the previous clock cycle. The `\$past' function is used to access the value of `edn\_req\_hold\_d' from the previous cycle. The `disable iff (~rst\_ni)' part ensures that the assertion is not checked when `rst\_ni' is low.
\end{tcolorbox}

In the base-model generated assertions, the chain of events depends on the reset signal, however, the assertion disables the `\texttt{rst\_ni}' signal. Moreover, the generated checking statement does not reflect the correct chain of events. `\texttt{edn\_req\_hold\_q}' should be assigned the current value of `\texttt{edn\_req\_hold\_d}', not the value it had in the previous clock cycle.

% \lstset{style=mystyle}
% \begin{lstlisting}[language=Verilog]
% Here is the requested property 

%  property ResetSynceotid; @(posedge clk_i) ( !rst_ni ) |-> edn_req_hold_q == '0 ;endproperty 
 
%  property SyncReqeotid; @(posedge clk_i) (  rst_ni ) |-> edn_req_hold_q == edn_req_hold_d ;endproperty
% \end{lstlisting}

\begin{tcolorbox}[colback=white, colframe=black, boxrule=0.2mm, sharp corners, title=DeepSeek Coder fine-tuned model response, coltitle=black, colbacktitle=white]
Here is the requested property 

\lstset{style=mystyle2}
\begin{lstlisting}[language=Verilog]
property ResetSynceotid; @(posedge clk_i) (!rst_ni)|-> edn_req_hold_q == '0; endproperty  
property SyncReqeotid; @(posedge clk_i) ( rst_ni)|->edn_req_hold_q==edn_req_hold_d; endproperty
\end{lstlisting}
\end{tcolorbox}

When generated by the same model fine-tuned on \dataset, it generates the assertions with `\texttt{rst\_ni}' under consideration, and it gets the correct clock cycle.

% \lstset{style=mystyle}
% \begin{lstlisting}[language=Verilog]
% <|begin_of_text|><|begin_of_text|><|start_header_id|>system<|end_header_id|>You are a helpful assistant. You are to analyze and generate the correct System Verilog Property for the given code <|eot_id|><|start_header_id|>user<|end_header_id|> Generate a list of synchronous systemverilog assertion executing at posedge clk_i from the following code 
%     if (!rst_ni) begin
%       lc_state_valid_q <= 1'b0;
%     end else begin
%       lc_state_valid_q <= lc_state_valid_d;
%     end

%  <|eot_id|><|start_header_id|>assistant<|end_header_id|>
% \end{lstlisting}

\begin{tcolorbox}[colback=white, colframe=black, boxrule=0.2mm, sharp corners, title=Llama 3.1 input prompt, coltitle=black, colbacktitle=white]
$<|eot\_id|><|start\_header\_id|>user<|end\_header\_id|>$ Generate a list of synchronous systemverilog assertion executing at posedge clk\_i from the following code:
\lstset{style=mystyle2}
\begin{lstlisting}[language=Verilog]
    if (!rst_ni) begin
      lc_state_valid_q <= 1'b0;
    end else begin
      lc_state_valid_q <= lc_state_valid_d;
    end
\end{lstlisting}
$<|eot\_id|><|start\_header\_id|>assistant<|end\_header\_id|>$
\end{tcolorbox}
% \lstset{style=mystyle}
% \begin{lstlisting}[language=Verilog]
% Here is the SystemVerilog property that corresponds to the given code:

% `property lc_state_valid_q_posedge;
%   @(posedge clk_i) ($rose(!rst_ni) |-> lc_state_valid_q === 1'b0) |-> lc_state_valid_q === lc_state_valid_d;
% endproperty`

% This property states that when the clock edge occurs, if the reset signal is asserted (i.e., `!rst_ni` is true), then `lc_state_valid_q` should be 0. If the reset signal is not asserted, then `lc_state_valid_q` should be equal to `lc_state_valid_d`. 

% Note that the `rose` function is used to check if the reset signal is asserted (i.e., goes from 0 to 1) at the current clock edge.
% \end{lstlisting}

\begin{tcolorbox}[colback=white, colframe=black, boxrule=0.2mm, sharp corners, title=Llama 3.1 base model response, coltitle=black, colbacktitle=white]
Here is the SystemVerilog property that corresponds to the given code:

\lstset{style=mystyle2}
\begin{lstlisting}[language=Verilog]
property lc_state_valid_q_posedge;
@(posedge clk_i) ($rose(!rst_ni)|->lc_state_valid_q===1'b0)|->lc_state_valid_q===lc_state_valid_d;
endproperty
\end{lstlisting}

This property states that when the clock edge occurs, if the reset signal is asserted (i.e., `!rst\_ni' is true), then `lc\_state\_valid\_q' should be 0. If the reset signal is not asserted, then `lc\_state\_valid\_q' should be equal to `lc\_state\_valid\_d'. 

Note that the `rose' function is used to check if the reset signal is asserted (i.e., goes from 0 to 1) at the current clock edge.
\end{tcolorbox}

Here, the base-model generated assertion does not get the chain of events right. The if-else block describes that if there is a reset invoked, `\texttt{lc\_state\_valid\_q}' is assigned $0$. Otherwise, it should be assigned the current value of `\texttt{lc\_state\_valid\_d}.' However, the generated assertion asserts that if `\texttt{!rst\_ni}' is risen, 
`\texttt{lc\_state\_valid\_q}' should be assigned $0$, and in the next clock cycle, it should be assigned `\texttt{lc\_state\_valid\_d}.' 

% \lstset{style=mystyle}
% \begin{lstlisting}[language=Verilog]
% property ResetSynceotid; @(posedge clk_i) (!rst_ni ) |-> lc_state_valid_q == 1'b0 ;endproperty 
 
% property ResetSynceotid; @(posedge clk_i)  ( rst_ni )  |-> lc_state_valid_q == lc_state_valid_d; endproperty 
% \end{lstlisting}

\begin{tcolorbox}[colback=white, colframe=black, boxrule=0.2mm, sharp corners, title=Llama 3.1 fine-tuned model response, coltitle=black, colbacktitle=white]
\lstset{style=mystyle2}
Here is the requested property
\begin{lstlisting}[language=Verilog]
property ResetSync1;@(posedge clk_i) (!rst_ni)|->lc_state_valid_q==1'b0; endproperty 
property ResetSync2;@(posedge clk_i) (rst_ni)|->lc_state_valid_q==lc_state_valid_d; endproperty 
\end{lstlisting}

\end{tcolorbox}

\subsubsection{CVA6 assertion examples}
\label{cva6_assert_examples}
\begin{tcolorbox}[colback=white, colframe=black, boxrule=0.2mm, sharp corners, title=DeepSeek Coder input prompt, coltitle=black, colbacktitle=white]
\#\#\# Instruction:Generate a list of asynchronous systemverilog assertion from the following code 
\lstset{style=mystyle2}
\begin{lstlisting}[language=Verilog]
 if (CVA6Cfg.RVH) begin
    if (CVA6Cfg.IS_XLEN64) begin : gen_vsstatus_64read
      assign vsstatus_extended = vsstatus_q[CVA6Cfg.XLEN-1:0];
    end else begin : gen_vsstatus_32read
      assign vsstatus_extended = {vsstatus_q.sd, vsstatus_q.wpri3[7:0], vsstatus_q[22:0]};
    end
  end else begin
    assign vsstatus_extended = '0;
  end
\end{lstlisting}
 \#\#\# Response: 
\end{tcolorbox}
% \lstset{style=mystyle}
% \begin{lstlisting}[language=Verilog]
% The given code is a synchronous systemverilog code for a flip-flop. It is a simple register that holds its value on the rising edge of the clock signal `clk_i`. The reset signal `rst_ni` is used to clear the register.

% The synchronous systemverilog assertion executing at posedge clk_i would be:

% ```systemverilog
% assert property (
%   @(posedge clk_i) disable iff (~rst_ni)
%     (edn_req_hold_q == $past(edn_req_hold_d, 1))
% );
% ```

% This assertion checks that the value of `edn_req_hold_q` is equal to the value of `edn_req_hold_d` at the previous clock cycle. The `$past` function is used to access the value of `edn_req_hold_d` from the previous cycle. The `disable iff (~rst_ni)` part ensures that the assertion is not checked when `rst_ni` is low.
% \end{lstlisting}

\begin{tcolorbox}[colback=white, colframe=black, boxrule=0.2mm, sharp corners, title= DeepSeek Coder base model response, coltitle=black, colbacktitle=white]
The code you provided is a SystemVerilog assertion. However, it does not contain any asynchronous assertions. Asynchronous assertions are used to check the conditions at different times. In your code, there are no conditions that would be checked asynchronously. 

If you want to create an asynchronous assertion, you would need to use the `\texttt{\$rose}' or `\texttt{\$fell}' functions to check for changes in the signal. However, this is not applicable in your code as there are no changes in the signal that you are checking.

Here is an example of an asynchronous assertion:

\lstset{style=mystyle2}
\begin{lstlisting}[language=Verilog]
always @(posedge clk or posedge reset) begin
  if (reset) begin
    // reset condition
  end
  else begin
    // check condition
    if ($rose(condition)) begin
      // do something
    end
  end
end
\end{lstlisting}

In this example, `\texttt{\$rose}(condition)' checks if `condition' rose (changed from 0 to 1) at the next clock edge.
\end{tcolorbox}

In this case, the base model generated an always block that does not assert anything.

% \lstset{style=mystyle}
% \begin{lstlisting}[language=Verilog]
% Here is the requested property 

%  property ResetSynceotid; @(posedge clk_i) ( !rst_ni ) |-> edn_req_hold_q == '0 ;endproperty 
 
%  property SyncReqeotid; @(posedge clk_i) (  rst_ni ) |-> edn_req_hold_q == edn_req_hold_d ;endproperty
% \end{lstlisting}

\begin{tcolorbox}[colback=white, colframe=black, boxrule=0.2mm, sharp corners, title=DeepSeek Coder fine-tuned model response, coltitle=black, colbacktitle=white]
Here is the requested property 

\lstset{style=mystyle2}
\begin{lstlisting}[language=Verilog]

  property ValidSynceotid; (CVA6Cfg.RVH) |-> (CVA6Cfg.IS_XLEN64) |-> vsstatus_extended == vsstatus_q[CVA6Cfg.XLEN-1:0] ;endproperty 
 
  property ValidSynceotid; (CVA6Cfg.RVH) |->  (CVA6Cfg.IS_XLEN64) |-> vsstatus_extended == {vsstatus_q.sd, vsstatus_q.wpri3[7:0], vsstatus_q[22:0]} ; endproperty 
 
  property SafeReseteotid; (CVA6Cfg.RVH) |-> vsstatus_extended == '0; endproperty
\end{lstlisting}
\end{tcolorbox}
%./RTL/CVA6/csr_regfile.sv
\begin{tcolorbox}[colback=white, colframe=black, boxrule=0.2mm, sharp corners, title=Llama 3.1 input prompt, coltitle=black, colbacktitle=white]
$<|start\_header\_id|>user<|end\_header\_id|>$ Generate a list of asynchronous systemverilog assertion from the following code 

\lstset{style=mystyle2}
\begin{lstlisting}[language=Verilog]
    if (CVA6Cfg.RVS) begin
      satp = satp_q;
    end
\end{lstlisting}
$<|eot\_id|><|start\_header\_id|>assistant<|end\_header\_id|>$
\end{tcolorbox}
\begin{tcolorbox}[colback=white, colframe=black, boxrule=0.2mm, sharp corners, title=Llama 3.1 base model response, coltitle=black, colbacktitle=white]
**Property: satp is updated when CVA6Cfg.RVS is asserted**

systemverilog
\lstset{style=mystyle2}
\begin{lstlisting}[language=Verilog]
property p_satp_updated;
  @(posedge clk) ($rose(CVA6Cfg.RVS) |=> satp === satp_q);
endproperty
\end{lstlisting}

\end{tcolorbox}

In this case, while the base model generated a syntactically correct property, it mistook the check condition as an edge-triggered event instead of a level-triggered event. Furthermore, it also got the clock cycle wrong. Instead of defining the property for the current clock cycle, it used the next clock cycle.

% \lstset{style=mystyle}
% \begin{lstlisting}[language=Verilog]
% property ResetSynceotid; @(posedge clk_i) (!rst_ni ) |-> lc_state_valid_q == 1'b0 ;endproperty 
 
% property ResetSynceotid; @(posedge clk_i)  ( rst_ni )  |-> lc_state_valid_q == lc_state_valid_d; endproperty 
% \end{lstlisting}

\begin{tcolorbox}[colback=white, colframe=black, boxrule=0.2mm, sharp corners, title=Llama 3.1 fine-tuned model response, coltitle=black, colbacktitle=white]
\lstset{style=mystyle2}
\begin{lstlisting}[language=Verilog]
 property SyncRegeotid; (CVA6Cfg.RVS) |-> satp == satp_q ;endproperty
\end{lstlisting}

\end{tcolorbox}

\subsubsection{Pulpissimo assertion examples}
\label{pulp_assert_examples}

\begin{tcolorbox}[colback=white, colframe=black, boxrule=0.2mm, sharp corners, title=DeepSeek Coder input prompt, coltitle=black, colbacktitle=white]
\#\#\# Instruction:Generate a list of asynchronous systemverilog assertion from the following code 
\lstset{style=mystyle2}
\begin{lstlisting}[language=Verilog]
    case (rdata_sel_q)
      RD_CSR:  debug_rdata_o = csr_rdata_i;
      RD_GPR:  debug_rdata_o = regfile_rdata_i;
      RD_DBGA: debug_rdata_o = dbg_rdata;
      RD_DBGS: debug_rdata_o = dbg_rdata;
    endcase
\end{lstlisting}
 \#\#\# Response: 
\end{tcolorbox}
% \lstset{style=mystyle}
% \begin{lstlisting}[language=Verilog]
% The given code is a synchronous systemverilog code for a flip-flop. It is a simple register that holds its value on the rising edge of the clock signal `clk_i`. The reset signal `rst_ni` is used to clear the register.

% The synchronous systemverilog assertion executing at posedge clk_i would be:

% ```systemverilog
% assert property (
%   @(posedge clk_i) disable iff (~rst_ni)
%     (edn_req_hold_q == $past(edn_req_hold_d, 1))
% );
% ```

% This assertion checks that the value of `edn_req_hold_q` is equal to the value of `edn_req_hold_d` at the previous clock cycle. The `$past` function is used to access the value of `edn_req_hold_d` from the previous cycle. The `disable iff (~rst_ni)` part ensures that the assertion is not checked when `rst_ni` is low.
% \end{lstlisting}

\begin{tcolorbox}[colback=white, colframe=black, boxrule=0.2mm, sharp corners, title= DeepSeek Coder base model response, coltitle=black, colbacktitle=white]
The code you provided is a SystemVerilog case statement. It seems like you want to generate a list of asynchronous assertions for this code. However, SystemVerilog does not support assertions in the same way as other languages (like C, Java, etc.). Assertions in SystemVerilog are used to check the design during compile time or run time.

If you want to generate asynchronous assertions, you would typically use the `\texttt{\$assertion\_off,}' `\texttt{\$assertion\_on},' `\texttt{\$assume},' `\texttt{\$cover},' or `\texttt{\$fell},' `\texttt{\$rose}' constructs.

However, without more context, it's hard to provide a more specific answer. If you could provide more information about the expected behavior or the conditions you want to check, I could give a more precise answer.

For example, if you want to ensure that `rdata\_sel\_q' is always valid (i.e., it's either `RD\_CSR,' `RD\_GPR,' `RD\_DBGA,' or `RD\_DBGS'), you could use an assertion like this:
\lstset{style=mystyle2}
\begin{lstlisting}[language=Verilog]
always @(*) begin
  $assert_on;
  assert (rdata_sel_q inside {RD_CSR, RD_GPR, RD_DBGA, RD_DBGS}) else $error("Invalid rdata_sel_q value");
end
\end{lstlisting}

\end{tcolorbox}

Here, the base model only checks whether the value of `\texttt{rdata\_sel\_q}' is within the defined parameters but not the operations.

% \lstset{style=mystyle}
% \begin{lstlisting}[language=Verilog]
% Here is the requested property 

%  property ResetSynceotid; @(posedge clk_i) ( !rst_ni ) |-> edn_req_hold_q == '0 ;endproperty 
 
%  property SyncReqeotid; @(posedge clk_i) (  rst_ni ) |-> edn_req_hold_q == edn_req_hold_d ;endproperty
% \end{lstlisting}

\begin{tcolorbox}[colback=white, colframe=black, boxrule=0.2mm, sharp corners, title=DeepSeek Coder fine-tuned model response, coltitle=black, colbacktitle=white]
Here is the requested property 

\lstset{style=mystyle2}
\begin{lstlisting}[language=Verilog]
property DataSynceotid; (rdata_sel_q)==(RD_DBGS)|->debug_rdata_o==dbg_rdata; endproperty 
property ValidRdeotid; (rdata_sel_q)==(RD_CSR)|->debug_rdata_o==csr_rdata_i; endproperty 
property ValidRdeotid; (rdata_sel_q)==(RD_GPR)|->debug_rdata_o==regfile_rdata_i; endproperty 
property ValidRdeotid; (rdata_sel_q)==(RD_DBGA)|->debug_rdata_o==dbg_rdata; endproperty 
\end{lstlisting}
\end{tcolorbox}

% \lstset{style=mystyle}
% \begin{lstlisting}[language=Verilog]
% <|begin_of_text|><|begin_of_text|><|start_header_id|>system<|end_header_id|>You are a helpful assistant. You are to analyze and generate the correct System Verilog Property for the given code <|eot_id|><|start_header_id|>user<|end_header_id|> Generate a list of synchronous systemverilog assertion executing at posedge clk_i from the following code 
%     if (!rst_ni) begin
%       lc_state_valid_q <= 1'b0;
%     end else begin
%       lc_state_valid_q <= lc_state_valid_d;
%     end

%  <|eot_id|><|start_header_id|>assistant<|end_header_id|>
% \end{lstlisting}

\begin{tcolorbox}[colback=white, colframe=black, boxrule=0.2mm, sharp corners, title=Llama 3.1 input prompt, coltitle=black, colbacktitle=white]
$<|eot\_id|><|start\_header\_id|>user<|end\_header\_id|>$ Generate a list of synchronous systemverilog assertion executing at posedge HCLK from the following code:
\lstset{style=mystyle2}
\begin{lstlisting}[language=Verilog]
        if(~HRESETn)
        begin
            r_status  <=  'h0;
        end
        else
        begin
            if (s_rise_int ) 
            begin
                r_status  <= r_status | s_is_int_all;
            end
            else if (PSEL && PENABLE &&!PWRITE && (s_apb_addr == `REG_INTSTATUS)) 
            begin
               r_status  <=  'h0;
            end
        end
    end
\end{lstlisting}
$<|eot\_id|><|start\_header\_id|>assistant<|end\_header\_id|>$
\end{tcolorbox}
% \lstset{style=mystyle}
% \begin{lstlisting}[language=Verilog]
% Here is the SystemVerilog property that corresponds to the given code:

% `property lc_state_valid_q_posedge;
%   @(posedge clk_i) ($rose(!rst_ni) |-> lc_state_valid_q === 1'b0) |-> lc_state_valid_q === lc_state_valid_d;
% endproperty`

% This property states that when the clock edge occurs, if the reset signal is asserted (i.e., `!rst_ni` is true), then `lc_state_valid_q` should be 0. If the reset signal is not asserted, then `lc_state_valid_q` should be equal to `lc_state_valid_d`. 

% Note that the `rose` function is used to check if the reset signal is asserted (i.e., goes from 0 to 1) at the current clock edge.
% \end{lstlisting}

\begin{tcolorbox}[colback=white, colframe=black, boxrule=0.2mm, sharp corners, title=Llama 3.1 base model response, coltitle=black, colbacktitle=white]
Here is the list of synchronous SystemVerilog assertions that can be generated from the given code, executing at posedge HCLK:
\lstset{style=mystyle2}

\begin{lstlisting}[language=Verilog]
property p_reset_default_value;
    @(posedge HCLK) disable iff (~HRESETn) $rose(r_status) == 1;
endproperty
\end{lstlisting}

\begin{lstlisting}[language=Verilog]
property p_int_status_set;
    @(posedge HCLK) disable iff (~HRESETn) (s_rise_int) |=> (r_status | s_is_int_all);
endproperty
\end{lstlisting}

\begin{lstlisting}[language=Verilog]
property p_apb_reset_int_status;
    @(posedge HCLK) disable iff (~HRESETn) (PSEL && PENABLE &&!PWRITE && (s_apb_addr == `REG_INTSTATUS)) |=> (r_status == 'h0);
endproperty
\end{lstlisting}

Note: The `disable iff` keyword is used to disable the property when the condition is false. The `rose` function is used to check if the value of `r\_status` has risen (i.e., changed from 0 to 1) at the current clock edge. The `|=>` operator is used to specify the implication relationship between the antecedent and the consequent.

\end{tcolorbox}

Here, the assertions miss the correct clock cycle for the assertions. Furthermore, it missed the nested conditional blocks under `\texttt{HRESETn},' which should have put the nested condition in an ``\texttt{AND}'' relation with `\texttt{HRESETn}.'

% \lstset{style=mystyle}
% \begin{lstlisting}[language=Verilog]
% property ResetSynceotid; @(posedge clk_i) (!rst_ni ) |-> lc_state_valid_q == 1'b0 ;endproperty 
 
% property ResetSynceotid; @(posedge clk_i)  ( rst_ni )  |-> lc_state_valid_q == lc_state_valid_d; endproperty 
% \end{lstlisting}

\begin{tcolorbox}[colback=white, colframe=black, boxrule=0.2mm, sharp corners, title=Llama 3.1 fine-tuned model response, coltitle=black, colbacktitle=white]
\lstset{style=mystyle2}
Here is the requested property 
\begin{lstlisting}[language=Verilog]
property ResetSync1; @(posedge clk_i) (!rst_ni)|->lc_state_valid_q==1'b0; endproperty 
property ResetSync2; @(posedge clk_i) (rst_ni)|->lc_state_valid_q==lc_state_valid_d; endproperty 
\end{lstlisting}

\end{tcolorbox}

\subsection{Difference between functional and syntactical assertions}
\label{diff_func_syn}

%%%%%%%%%%%%%%%%%%%%%%%%%%%%%%%%%%%%%%%%%%%%%%%%%%%%%%%%%%%%%%%%%%%%%%%%%%%%%%%%%%%

\begin{tcolorbox}[colback=white, colframe=black, boxrule=0.2mm, sharp corners, title={Syntactical and Functional Errors in Assertions.}, coltitle=black, colbacktitle=white]
\lstset{style=mystyle2}
\label{tb:diff_func_syn}

Design Source Code:

\begin{lstlisting}[language=Verilog]
always_ff @(posedge clk_aon_i or negedge rst_aon_ni) begin
    if (!rst_aon_ni) begin
        wakeup_timer_cnt_q    <= '0;
    end
    else if (wakeup_timer_cnt_clr || cfg_fsm_rst_i || trigger_h2l) begin
        wakeup_timer_cnt_q <= '0;
    end else begin
        wakeup_timer_cnt_q <= wakeup_timer_cnt_d;
    end
end
\end{lstlisting}

Here is the requested property 
\begin{lstlisting}[language=Verilog]
property ResetTimer1; @(posedge clk_aon_i) (!rst_aon_ni)|->wakeup_timer_cnt_q=1'b0; endproperty 
// A syntactically incorrect assertion
// Here, instead of using `==' symbol, `=' was used
property ResetTimer2;
@(posedge clk_aon_i)(wakeup_timer_cnt_clr||cfg_fsm_rst_i||trigger_h2l)|->wakeup_timer_cnt_q=='0;
endproperty
// A Functionally incorrect assertion
// Here, the generated assertion is missed capturing the `if' condition.
\end{lstlisting}

\end{tcolorbox}

%%%%%%%%%%%%%%%%%%%%%%%%%%%%%%%%%%%%%%%%%%%%%%%%%%%%%%%%%%%%%%%%%%%%%%%%%%%%%%%%%%%

Since formal tools like \cite{jasper} assume that asynchronous reset signals remain inactive during execution \cite{miftah2024system}, we use simulation in \cite{vivado} to verify assertions involving asynchronous resets and ensure the asserted properties can be covered. Next, we validate the functional correctness of the assertions by performing formal and simulation verification runs, validating that the assertions can be triggered and observed during testing. This two-stage process ensures that only syntactically correct and functionally valid assertions are retained in the design. Textbox \ref{tb:diff_func_syn} illustrates the difference between syntactical and functional errors in assertions within a hardware design context. It presents two issues that can arise when writing assertions to verify system behavior.

\paragraph{Design Source Code:}
The provided SystemVerilog code shows an \texttt{always\_ff} block, triggered by either the rising edge of \texttt{clk\_aon\_i} or the falling edge of \texttt{rst\_aon\_ni}. The block resets or updates the value of \texttt{wakeup\_timer\_cnt\_q} based on certain conditions:
\begin{enumerate}
    \item If \texttt{rst\_aon\_ni} is low (reset active), the counter is set to zero.
    \item If \texttt{wakeup\_timer\_cnt\_clr} or certain other signals are asserted, the counter is reset.
    \item Otherwise, the counter is updated with a new value from \texttt{wakeup\_timer\_cnt\_d}.
\end{enumerate}

\paragraph{Assertions:}
Two properties are presented, each demonstrating a different type of error:

\begin{itemize}
    \item \textbf{Syntactical Error:} \\
    In \texttt{property ResetTimer1}, the assertion attempts to check if the counter is reset when \texttt{rst\_aon\_ni} is low. However, it contains a \textbf{syntactical error}: instead of using the comparison operator \texttt{==} to check if \texttt{wakeup\_timer\_cnt\_q} equals zero, the assignment operator \texttt{=} is mistakenly used. This would result in a syntax error during compilation.
    
    \item \textbf{Functional Error:} \\
    In \texttt{property ResetTimer2}, while the syntax is correct, the assertion misses an essential condition. It checks whether the counter is reset when the clear signal or related signals are asserted. However, it fails to include the reset condition (i.e., \texttt{if (!rst\_aon\_ni)}), resulting in a \textbf{functional error} because the assertion does not fully capture the intended behavior of the design, specifically missing the \texttt{if} condition from the original source code.
\end{itemize}

\paragraph{Key Point:}
We highlight how both types of errors (syntactical and functional) can undermine the correctness of assertions, either by preventing successful compilation (in the case of syntax errors) or by failing to accurately verify the design's intended behavior (in the case of functional errors).

%% REBUTTAL ADDED STUFF

\subsection{Examples of LLMs Fine-tuned on VERT Addressing GPT-4o Issues and Comparison With Human Experts}
\textcolor{blue}{In this section, we show how the intuition in dataset formulation, as discussed in Section 4.1 of our paper, translates into the effectiveness of the assertions generated by LLMs fine-tuned on VERT. Furthermore, we also provide a comparison of these models with human experts. These scenarios include (1) clock cycle and pre-condition capturing, (2) relation representation for nested conditional blocks, and (3) handling long conditions. Each section begins with the relevant code snippet, followed by the assertions generated by each approach.}

\input{Appendix_exmaples_Addressing_Issues/Clock_cycle}

\subsubsection{ LLMs Fine-tuned on VERT vs. GPT-4o:} 
\label{vertvsgpt4}

\textcolor{blue}{\textbf{Clock Cycle Misinterpretations:} We observe that LLMs often get confused between using the overlapping implication symbol ($|->$) and the non-overlapping symbol ($|=>$). To resolve clock cycle misinterpretation by LLMs, we standardized our format by using the overlapping implication symbol with a specified delay count and replacing the non-overlapping symbol. As shown in text box \ref{tbox:sv_clkcycle_appn} below, GPT-4o incorrectly uses the non-overlapping symbol, but both LLMs fine-tuned on VERT address this issue by correctly interpreting the clock cycle by using the overlapping implication symbol.}

\textcolor{blue}{\textbf{Miscapturing if Condition for else Branches:} LLMs often overlook the previous if/else if conditions when generating assertions for the subsequent else or else if branches in conditional statements. VERT addresses the common omission of conditions in the else/else-if branches of if-else statements by exposing the model to diverse conditional structures. As shown in text box \ref{tbox:sv_nestedIF_appn} below,  GPT-4o, in its second assertion, misses that the second assertion should verify that $monitor\_enable$ is \textit{FALSE} and $monitor\_enable\_q$ is \textit{TRUE}. However, both LLMs fine-tuned on VERT correctly identify these conditions and include them in the fourth generated assertion.}

\input{Appendix_exmaples_Addressing_Issues/nested_if}

\textcolor{blue}{\textbf{Nested If-Else Conditions:} LLMs often struggle with generating assertions for deeply nested if-else conditions (i.e., blocks nested beyond two levels), which are common in hardware design. To address the challenge of LLMs struggling with deeply nested if-else statements, we expanded VERT to include complex, multi-level conditional structures. As illustrated by text box \ref{tbox:sv_nestedIF_appn} below, GPT-4o incorrectly represents the logic of a nested block. Specifically, it ignores the if condition and creates an assertion using a ternary operator, where the inner if condition is used as the test, the assignment is the \textit{TRUE} branch, and \textit{1'b1} is the \textit{TRUE} branch. However, both LLMs fine-tuned on VERT to correctly identify the correct nested statement and their conditions.}

\input{Appendix_exmaples_Addressing_Issues/Long_Conditions}

\textcolor{blue}{\textbf{Handling Long Conditions:} To address the challenge of generating accurate assertions for long and complex conditions, we expanded VERT to include a variety of cases where multiple conditions and operators must be evaluated simultaneously. As shown in text box \ref{tbox:sv_long_appn} below, the source code requires any one of six conditions to be met before raising the $mr\_err$ flag. However, the generated output by GPT- 4o creates three assertions for one flag change, each neglecting the other three conditions. This not only leads to incorrect assertions but also causes overhead in the number of assertions. However, both LLMs fine-tuned on VERT correctly generate a singular assertion that describes all the conditions and their relationships within the if-statement.}

\subsubsection{ LLMs Fine-tuned on VERT vs. Human Expert:} 

{\color{blue}
Human experts and LLMs fine-tuned on VERT generate assertions differently. Experts often create simpler, more readable assertions, reflecting a preference for human-friendly formats. LLMs, on the other hand, produce more standardized logical expressions. This difference highlights style preferences rather than superiority. Notably, despite these stylistic differences, LLMs fine-tuned on VERT achieve assertion generation performance comparable to that of human experts. This is illustrated in the textbox \ref{tbox:hum_exp}. 
For instance, in example 1, when verifying whether the \texttt{bus\_release\_cnt} signal has been reset, the LLM-generated assertion takes the form \texttt{bus\_release\_cnt == '0'}, while the human expert expresses the same operation as \texttt{!(|bus\_release\_cnt)}. The latter format, often favored by experts, is typically chosen for its ease of writing and brevity. Similarly, in example 2, since \textit{mr\_err} is a one-bit flag, the human expert chooses to verify whether the flag was raised by writing \texttt{mr\_err} for the check, while the LLMs use the full expression, \texttt{mr\_err == 1'b1}.
}

% TO DO Explain 2 and 3

\input{Appendix_exmaples_Addressing_Issues/HumanExpert}
\input{Tables/abl_table}

% \newpage
\subsection{Ablation Study with Uncleaned Variable Names}

\textcolor{blue}{Table \ref{tab:abl_table} an ablation study with uncleaned variable names, presented below, to highlight the impact of cleaning variable names. The Table is split into two halves, containing Syntactically Correct Assertions and Functionally Correct Assertions. Columns 3 and 8 refer to the assertions generated by the base model. Columns 4 and 9 refer to assertions generated by a model fine-tuned on a dataset that contains syntactically incorrect variables (which refer to special characters not allowed in HDL languages); columns 5 and 10 refer to duplicate variables that may skew the model’s learning and introduce ambiguity, and columns 6 and 11 refer to inconsistent variables such as conflicting variable names. Finally, columns 7 and 12 refer to the cleaned variables we eventually use to build VERT. The results provided in the table below demonstrate that failing to address syntactically incorrect variable names was the most critical, leading to lower performance in fine-tuned LLMs compared to even the base models. This is because the fine-tuned LLMs generate syntactically incorrect assertions stemming from erroneous variable names.}

\textcolor{blue}{Subsequently, LLMs fine-tuned with the cleaned variable list (VERT) performed up to 17.76\% and  17.39\% in syntactical and functional correctness, respectively, compared to the LLMs fine-tuned on a dataset that preserved duplicate variable names. This improvement is attributed to eliminating duplicates within the same assertion, which likely reduced ambiguity and enhanced the fine-tuned LLMs' ability to generate accurate results.
Finally, addressing inconsistent variable names resulted in the smallest observed change, with the LLMs fine-tuned on the cleaned variable list increasing by up to 3.24\% and 4.81\%, in syntactical and functional correctness, respectively, compared to the LLMs fine-tuned on a dataset that maintained inconsistent variable names. This outcome is likely because such inconsistencies comprised a relatively minor portion of the overall variable list compared to the duplicates and syntactically incorrect variables.}

\subsection{Evaluating Impact of Contamination on Assertion Generation}

\input{Tables/contamination}

\textcolor{blue}{Regarding potential data contamination, from our experiments, we observed that certain HDL components negatively impact the generation of syntactically and functionally correct assertions. Notably, module instantiations and ``ifdef” commands challenge assertion generation. Specifically, the models used to evaluate VERT rarely generate assertions from module instantiations, leading to syntactically and functionally incorrect results.
Moreover, these smaller models tend to misinterpret ``ifdef” commands as conventional if-else statements. While this misclassification occurs infrequently, it reduces the percentage of correctly generated assertions. Assertions derived from these commands are often both syntactically incorrect—since ``ifdef” commands do not adhere to standard if-else syntax and lack the necessary information for typical branching—and functionally incorrect, as they do not contribute meaningfully to functional branching. In contrast, GPT-4o appears unaffected by these HDL components in its assertion generation.
Table 1 illustrates the effect of increasing contamination in design files on assertion generation. Here, ``contamination” refers to adding ``ifdef” commands and module instantiations. For example, ``+10 contamination” indicates that 10 additional instances of each of these elements (on top of the already existing instances) were introduced into the design files. The results show that as the level of contamination increases, the number of incorrectly generated assertions also rises. It should be noted that typically, in the hardware design, the number of ``ifdef” commands is limited to at most five. Therefore, the scenarios used here to evaluate the contamination effect are unrealistic and to study the effect of contamination on the models.}

\textcolor{blue}{Table \ref{tab:cont-table} illustrates the effect of increasing contamination in design files on assertion generation. Column 1, ``Models," specifies the LLM being tested, while Column 2, ``Benchmark/Hardware IP," lists the specific test benchmark used. Columns 3, 4, and 5, under ``Generated Assertions," indicate the total number of assertions generated with no contamination, an additional 10 contamination, and an additional 20 contamination in the input dataset, respectively. Columns 6, 7, and 8, under ``Syntactically Correct (\%)," measure the percentage of assertions that are syntactically valid for each contamination level. Finally, Columns 9, 10, and 11, under ``Functionally Correct (\%)," represent the percentage of assertions that are logically accurate and align with the intended functionality under the same contamination conditions. Here, ``contamination” refers to the addition of ``ifdef” commands and module instantiations. A contamination level lower than 10 was found to have a negligible impact on the results, while levels exceeding 20 were impractical due to exceeding the context size limitations of our models. The results show that as the level of contamination increases, the number of incorrectly generated assertions also rises. This results in a 3\% drop in accuracy.  It should be noted that typically, in the hardware design, the number of ``ifdef” commands is limited to at most five. Therefore, the scenarios used here to evaluate the contamination effect are unrealistic and for the purpose of studying the effect of contamination on the models.}

\subsection{Assessing Functional Correctness and Relevance of Assertions through Mutation Testing}
\label{mutation}

\textcolor{blue}{The functional correctness of the generated assertions, as presented in Table \ref{tab:asserttable}, was evaluated using mutation testing, consistent with the methodology outlined in [1]. This approach involved introducing intentional, small code modifications (mutants) that deviated from the expected assertion logic. By detecting these mutants, we demonstrated the effectiveness of the generated assertions in identifying logical inconsistencies and validating their utility. Unlike trivial or redundant assertions (e.g., ``assert True"), these assertions were intricately aligned with the critical components of the hardware design, ensuring their relevance and impact.
Our findings revealed that the generated assertions achieved up to 100\% functional correctness or ability to detect mutations across various benchmarks, underscoring their robustness and effectiveness. The same mutation testing methodology from [1] was also applied to verify the importance of the generated assertions, further affirming their significance. This comprehensive evaluation highlighted the non-redundant nature of the benchmarks and the potential of LLMs fine-tuned on VERT for hardware verification. Furthermore, the method ensured complete coverage of conditional branches and critical logic paths within the hardware design. The LLM-generated assertions were specifically crafted to validate every logical path, leaving no branch or condition unchecked, thereby reinforcing their role in achieving thorough hardware verification.}

\subsection{Coverage Measurement}
\label{sec:coverage_measurement_appen}
\textcolor{blue}{Complete Path Coverage (CPC) refers to covering all possible independent paths within an automaton. A path begins at the initial node, traverses through the graph's edges, and ends at a final node. While CPC provides a thorough examination of the system, it becomes infeasible for graphs containing cycles, as these can result in infinite path lengths.}

\textcolor{blue}{In our approach, we use complete path coverage as our primary coverage metric. This ensures a comprehensive evaluation of the system's behavior by accounting for all potential paths. To validate our coverage, we employed both formal and simulation-based verification tools, including \cite{jasper} and \cite{vivado}. These tools allowed us to rigorously analyze the generated assertions and ensure that they comprehensively cover all the functions defined within the system.}

\textcolor{blue}{By leveraging our method to extract properties from every possible conditional branch, we achieve up to 100\% coverage. This robust verification strategy confirms the correctness and reliability of the automaton's functionality across all defined behaviors.}
