# Supplementary material for: Enhancing Large Language Models for Hardware Verification: A Novel SystemVerilog Assertion Dataset
Source: arXiv:2503.08923 source file (2025-03-11)
Supplement: Supplementary file 2 [file CODE_for_LLAMA3.tex]

%./RTL/CVA6/csr_regfile.sv
\begin{tcolorbox}[colback=white, colframe=black, boxrule=0.2mm, sharp corners, title=Llama 3.1 input prompt, coltitle=black, colbacktitle=white]
$<|start\_header\_id|>user<|end\_header\_id|>$ Generate a list of asynchronous systemverilog assertion from the following code 

\lstset{style=mystyle2}
\begin{lstlisting}[language=Verilog]
    if (CVA6Cfg.RVS) begin
      satp = satp_q;
    end
\end{lstlisting}
$<|eot\_id|><|start\_header\_id|>assistant<|end\_header\_id|>$
\end{tcolorbox}
