# Supplementary material for: Enhancing Large Language Models for Hardware Verification: A Novel SystemVerilog Assertion Dataset
Source: arXiv:2503.08923 source file (2025-03-11)
Supplement: Supplementary file 3 [file Code_for_DEEPSEEK.tex]

\begin{tcolorbox}[colback=white, colframe=black, boxrule=0.2mm, sharp corners, title=DeepSeek Coder input prompt, coltitle=black, colbacktitle=white]
\#\#\# Instruction:Generate a list of asynchronous systemverilog assertion from the following code 
\lstset{style=mystyle2}
\begin{lstlisting}[language=Verilog]
 if (CVA6Cfg.RVH) begin
    if (CVA6Cfg.IS_XLEN64) begin : gen_vsstatus_64read
      assign vsstatus_extended = vsstatus_q[CVA6Cfg.XLEN-1:0];
    end else begin : gen_vsstatus_32read
      assign vsstatus_extended = {vsstatus_q.sd, vsstatus_q.wpri3[7:0], vsstatus_q[22:0]};
    end
  end else begin
    assign vsstatus_extended = '0;
  end
\end{lstlisting}
 \#\#\# Response: 
\end{tcolorbox}
