# Supplementary material for: Enhancing Large Language Models for Hardware Verification: A Novel SystemVerilog Assertion Dataset
Source: arXiv:2503.08923 source file (2025-03-11)
Supplement: Supplementary file 4 [file Deepseek_example_listing.tex]

% \lstset{style=mystyle}
% \begin{lstlisting}[language=Verilog]
% Here is the requested property 

%  property ResetSynceotid; @(posedge clk_i) ( !rst_ni ) |-> edn_req_hold_q == '0 ;endproperty 
 
%  property SyncReqeotid; @(posedge clk_i) (  rst_ni ) |-> edn_req_hold_q == edn_req_hold_d ;endproperty
% \end{lstlisting}

\begin{tcolorbox}[colback=white, colframe=black, boxrule=0.2mm, sharp corners, title=DeepSeek Coder fine-tuned model response, coltitle=black, colbacktitle=white]
Here is the requested property 

\lstset{style=mystyle2}
\begin{lstlisting}[language=Verilog]

  property ValidSynceotid; (CVA6Cfg.RVH) |-> (CVA6Cfg.IS_XLEN64) |-> vsstatus_extended == vsstatus_q[CVA6Cfg.XLEN-1:0] ;endproperty 
 
  property ValidSynceotid; (CVA6Cfg.RVH) |->  (CVA6Cfg.IS_XLEN64) |-> vsstatus_extended == {vsstatus_q.sd, vsstatus_q.wpri3[7:0], vsstatus_q[22:0]} ; endproperty 
 
  property SafeReseteotid; (CVA6Cfg.RVH) |-> vsstatus_extended == '0; endproperty
\end{lstlisting}
\end{tcolorbox}
