# Supplementary material for: Enhancing Large Language Models for Hardware Verification: A Novel SystemVerilog Assertion Dataset
Source: arXiv:2503.08923 source file (2025-03-11)
Supplement: Supplementary file 5 [file Deepseek_example_listing_ND.tex]

% \lstset{style=mystyle}
% \begin{lstlisting}[language=Verilog]
% The given code is a synchronous systemverilog code for a flip-flop. It is a simple register that holds its value on the rising edge of the clock signal `clk_i`. The reset signal `rst_ni` is used to clear the register.

% The synchronous systemverilog assertion executing at posedge clk_i would be:

% ```systemverilog
% assert property (
%   @(posedge clk_i) disable iff (~rst_ni)
%     (edn_req_hold_q == $past(edn_req_hold_d, 1))
% );
% ```

% This assertion checks that the value of `edn_req_hold_q` is equal to the value of `edn_req_hold_d` at the previous clock cycle. The `$past` function is used to access the value of `edn_req_hold_d` from the previous cycle. The `disable iff (~rst_ni)` part ensures that the assertion is not checked when `rst_ni` is low.
% \end{lstlisting}

\begin{tcolorbox}[colback=white, colframe=black, boxrule=0.2mm, sharp corners, title= DeepSeek Coder base model response, coltitle=black, colbacktitle=white]
The code you provided is a SystemVerilog assertion. However, it does not contain any asynchronous assertions. Asynchronous assertions are used to check the conditions at different times. In your code, there are no conditions that would be checked asynchronously. 

If you want to create an asynchronous assertion, you would need to use the `\texttt{\$rose}' or `\texttt{\$fell}' functions to check for changes in the signal. However, this is not applicable in your code as there are no changes in the signal that you are checking.

Here is an example of an asynchronous assertion:

\lstset{style=mystyle2}
\begin{lstlisting}[language=Verilog]
always @(posedge clk or posedge reset) begin
  if (reset) begin
    // reset condition
  end
  else begin
    // check condition
    if ($rose(condition)) begin
      // do something
    end
  end
end
\end{lstlisting}

In this example, `\texttt{\$rose}(condition)' checks if `condition' rose (changed from 0 to 1) at the next clock edge.
\end{tcolorbox}
