# Supplementary material for: Enhancing Large Language Models for Hardware Verification: A Novel SystemVerilog Assertion Dataset
Source: arXiv:2503.08923 source file (2025-03-11)
Supplement: Supplementary file 6 [file LLama3_example_listing.tex]

% \lstset{style=mystyle}
% \begin{lstlisting}[language=Verilog]
% property ResetSynceotid; @(posedge clk_i) (!rst_ni ) |-> lc_state_valid_q == 1'b0 ;endproperty 
 
% property ResetSynceotid; @(posedge clk_i)  ( rst_ni )  |-> lc_state_valid_q == lc_state_valid_d; endproperty 
% \end{lstlisting}

\begin{tcolorbox}[colback=white, colframe=black, boxrule=0.2mm, sharp corners, title=Llama 3.1 fine-tuned model response, coltitle=black, colbacktitle=white]
\lstset{style=mystyle2}
\begin{lstlisting}[language=Verilog]
 property SyncRegeotid; (CVA6Cfg.RVS) |-> satp == satp_q ;endproperty
\end{lstlisting}

\end{tcolorbox}
