# Supplementary material for: Enhancing Large Language Models for Hardware Verification: A Novel SystemVerilog Assertion Dataset
Source: arXiv:2503.08923 source file (2025-03-11)
Supplement: Supplementary file 7 [file LLama3_example_listing_ND.tex]

\begin{tcolorbox}[colback=white, colframe=black, boxrule=0.2mm, sharp corners, title=Llama 3.1 base model response, coltitle=black, colbacktitle=white]
**Property: satp is updated when CVA6Cfg.RVS is asserted**

systemverilog
\lstset{style=mystyle2}
\begin{lstlisting}[language=Verilog]
property p_satp_updated;
  @(posedge clk) ($rose(CVA6Cfg.RVS) |=> satp === satp_q);
endproperty
\end{lstlisting}

\end{tcolorbox}
