# Supplementary material for: Enhancing Large Language Models for Hardware Verification: A Novel SystemVerilog Assertion Dataset
Source: arXiv:2503.08923 source file (2025-03-11)
Supplement: Supplementary file 8 [file CODE_for_LLAMA3.tex]

% \lstset{style=mystyle}
% \begin{lstlisting}[language=Verilog]
% <|begin_of_text|><|begin_of_text|><|start_header_id|>system<|end_header_id|>You are a helpful assistant. You are to analyze and generate the correct System Verilog Property for the given code <|eot_id|><|start_header_id|>user<|end_header_id|> Generate a list of synchronous systemverilog assertion executing at posedge clk_i from the following code 
%     if (!rst_ni) begin
%       lc_state_valid_q <= 1'b0;
%     end else begin
%       lc_state_valid_q <= lc_state_valid_d;
%     end

%  <|eot_id|><|start_header_id|>assistant<|end_header_id|>
% \end{lstlisting}

\begin{tcolorbox}[colback=white, colframe=black, boxrule=0.2mm, sharp corners, title=Llama 3.1 input prompt, coltitle=black, colbacktitle=white]
$<|eot\_id|><|start\_header\_id|>user<|end\_header\_id|>$ Generate a list of synchronous systemverilog assertion executing at posedge clk\_i from the following code:
\lstset{style=mystyle2}
\begin{lstlisting}[language=Verilog]
    if (!rst_ni) begin
      lc_state_valid_q <= 1'b0;
    end else begin
      lc_state_valid_q <= lc_state_valid_d;
    end
\end{lstlisting}
$<|eot\_id|><|start\_header\_id|>assistant<|end\_header\_id|>$
\end{tcolorbox}
