# Supplementary material for: Enhancing Large Language Models for Hardware Verification: A Novel SystemVerilog Assertion Dataset
Source: arXiv:2503.08923 source file (2025-03-11)
Supplement: Supplementary file 9 [file Code_for_DEEPSEEK.tex]

\begin{tcolorbox}[colback=white, colframe=black, boxrule=0.2mm, sharp corners, title=DeepSeek Coder input prompt, coltitle=black, colbacktitle=white]
\#\#\# Instruction: Generate a list of synchronous SystemVerilog assertions executing at posedge clk\_i from the following code: 
\lstset{style=mystyle2}
\begin{lstlisting}[language=Verilog]
    if (!rst_ni) begin
      edn_req_hold_q <= '0;
    end else begin
      edn_req_hold_q <= edn_req_hold_d;
    end
\end{lstlisting}
 \#\#\# Response: 
\end{tcolorbox}
