# Supplementary material for: Enhancing Large Language Models for Hardware Verification: A Novel SystemVerilog Assertion Dataset
Source: arXiv:2503.08923 source file (2025-03-11)
Supplement: Supplementary file 11 [file Deepseek_example_listing_ND.tex]

% \lstset{style=mystyle}
% \begin{lstlisting}[language=Verilog]
% The given code is a synchronous systemverilog code for a flip-flop. It is a simple register that holds its value on the rising edge of the clock signal `clk_i`. The reset signal `rst_ni` is used to clear the register.

% The synchronous systemverilog assertion executing at posedge clk_i would be:

% ```systemverilog
% assert property (
%   @(posedge clk_i) disable iff (~rst_ni)
%     (edn_req_hold_q == $past(edn_req_hold_d, 1))
% );
% ```

% This assertion checks that the value of `edn_req_hold_q` is equal to the value of `edn_req_hold_d` at the previous clock cycle. The `$past` function is used to access the value of `edn_req_hold_d` from the previous cycle. The `disable iff (~rst_ni)` part ensures that the assertion is not checked when `rst_ni` is low.
% \end{lstlisting}

\begin{tcolorbox}[colback=white, colframe=black, boxrule=0.2mm, sharp corners, title= DeepSeek Coder base model response, coltitle=black, colbacktitle=white]
The given code is a synchronous systemverilog code for a flip-flop. It is a simple register that holds its value on the rising edge of the clock signal `clk\_i'. The reset signal `rst\_ni' is used to clear the register.

The synchronous systemverilog assertion executing at posedge clk\_i would be:

% \vspace{2mm}\textbf{SystemVerilog:}
\lstset{style=mystyle2}
\begin{lstlisting}[language=Verilog]
assert property (
  @(posedge clk_i) disable iff (~rst_ni)
    (edn_req_hold_q == $past(edn_req_hold_d, 1))
);
\end{lstlisting}

This assertion checks that the value of `edn\_req\_hold\_q' is equal to the value of `edn\_req\_hold\_d' at the previous clock cycle. The `\$past' function is used to access the value of `edn\_req\_hold\_d' from the previous cycle. The `disable iff (~rst\_ni)' part ensures that the assertion is not checked when `rst\_ni' is low.
\end{tcolorbox}
