# Supplementary material for: Enhancing Large Language Models for Hardware Verification: A Novel SystemVerilog Assertion Dataset
Source: arXiv:2503.08923 source file (2025-03-11)
Supplement: Supplementary file 13 [file LLama3_example_listing_ND.tex]

% \lstset{style=mystyle}
% \begin{lstlisting}[language=Verilog]
% Here is the SystemVerilog property that corresponds to the given code:

% `property lc_state_valid_q_posedge;
%   @(posedge clk_i) ($rose(!rst_ni) |-> lc_state_valid_q === 1'b0) |-> lc_state_valid_q === lc_state_valid_d;
% endproperty`

% This property states that when the clock edge occurs, if the reset signal is asserted (i.e., `!rst_ni` is true), then `lc_state_valid_q` should be 0. If the reset signal is not asserted, then `lc_state_valid_q` should be equal to `lc_state_valid_d`. 

% Note that the `rose` function is used to check if the reset signal is asserted (i.e., goes from 0 to 1) at the current clock edge.
% \end{lstlisting}

\begin{tcolorbox}[colback=white, colframe=black, boxrule=0.2mm, sharp corners, title=Llama 3.1 base model response, coltitle=black, colbacktitle=white]
Here is the SystemVerilog property that corresponds to the given code:

\lstset{style=mystyle2}
\begin{lstlisting}[language=Verilog]
property lc_state_valid_q_posedge;
@(posedge clk_i) ($rose(!rst_ni)|->lc_state_valid_q===1'b0)|->lc_state_valid_q===lc_state_valid_d;
endproperty
\end{lstlisting}

This property states that when the clock edge occurs, if the reset signal is asserted (i.e., `!rst\_ni' is true), then `lc\_state\_valid\_q' should be 0. If the reset signal is not asserted, then `lc\_state\_valid\_q' should be equal to `lc\_state\_valid\_d'. 

Note that the `rose' function is used to check if the reset signal is asserted (i.e., goes from 0 to 1) at the current clock edge.
\end{tcolorbox}
