# Supplementary material for: Enhancing Large Language Models for Hardware Verification: A Novel SystemVerilog Assertion Dataset
Source: arXiv:2503.08923 source file (2025-03-11)
Supplement: Supplementary file 15 [file Code_for_DEEPSEEK.tex]

\begin{tcolorbox}[colback=white, colframe=black, boxrule=0.2mm, sharp corners, title=DeepSeek Coder input prompt, coltitle=black, colbacktitle=white]
\#\#\# Instruction:Generate a list of asynchronous systemverilog assertion from the following code 
\lstset{style=mystyle2}
\begin{lstlisting}[language=Verilog]
    case (rdata_sel_q)
      RD_CSR:  debug_rdata_o = csr_rdata_i;
      RD_GPR:  debug_rdata_o = regfile_rdata_i;
      RD_DBGA: debug_rdata_o = dbg_rdata;
      RD_DBGS: debug_rdata_o = dbg_rdata;
    endcase
\end{lstlisting}
 \#\#\# Response: 
\end{tcolorbox}
