# Supplementary material for: Enhancing Large Language Models for Hardware Verification: A Novel SystemVerilog Assertion Dataset
Source: arXiv:2503.08923 source file (2025-03-11)
Supplement: Supplementary file 16 [file Deepseek_example_listing.tex]

% \lstset{style=mystyle}
% \begin{lstlisting}[language=Verilog]
% Here is the requested property 

%  property ResetSynceotid; @(posedge clk_i) ( !rst_ni ) |-> edn_req_hold_q == '0 ;endproperty 
 
%  property SyncReqeotid; @(posedge clk_i) (  rst_ni ) |-> edn_req_hold_q == edn_req_hold_d ;endproperty
% \end{lstlisting}

\begin{tcolorbox}[colback=white, colframe=black, boxrule=0.2mm, sharp corners, title=DeepSeek Coder fine-tuned model response, coltitle=black, colbacktitle=white]
Here is the requested property 

\lstset{style=mystyle2}
\begin{lstlisting}[language=Verilog]
property DataSynceotid; (rdata_sel_q)==(RD_DBGS)|->debug_rdata_o==dbg_rdata; endproperty 
property ValidRdeotid; (rdata_sel_q)==(RD_CSR)|->debug_rdata_o==csr_rdata_i; endproperty 
property ValidRdeotid; (rdata_sel_q)==(RD_GPR)|->debug_rdata_o==regfile_rdata_i; endproperty 
property ValidRdeotid; (rdata_sel_q)==(RD_DBGA)|->debug_rdata_o==dbg_rdata; endproperty 
\end{lstlisting}
\end{tcolorbox}
