# Supplementary material for: Enhancing Large Language Models for Hardware Verification: A Novel SystemVerilog Assertion Dataset
Source: arXiv:2503.08923 source file (2025-03-11)
Supplement: Supplementary file 17 [file Deepseek_example_listing_ND.tex]

% \lstset{style=mystyle}
% \begin{lstlisting}[language=Verilog]
% The given code is a synchronous systemverilog code for a flip-flop. It is a simple register that holds its value on the rising edge of the clock signal `clk_i`. The reset signal `rst_ni` is used to clear the register.

% The synchronous systemverilog assertion executing at posedge clk_i would be:

% ```systemverilog
% assert property (
%   @(posedge clk_i) disable iff (~rst_ni)
%     (edn_req_hold_q == $past(edn_req_hold_d, 1))
% );
% ```

% This assertion checks that the value of `edn_req_hold_q` is equal to the value of `edn_req_hold_d` at the previous clock cycle. The `$past` function is used to access the value of `edn_req_hold_d` from the previous cycle. The `disable iff (~rst_ni)` part ensures that the assertion is not checked when `rst_ni` is low.
% \end{lstlisting}

\begin{tcolorbox}[colback=white, colframe=black, boxrule=0.2mm, sharp corners, title= DeepSeek Coder base model response, coltitle=black, colbacktitle=white]
The code you provided is a SystemVerilog case statement. It seems like you want to generate a list of asynchronous assertions for this code. However, SystemVerilog does not support assertions in the same way as other languages (like C, Java, etc.). Assertions in SystemVerilog are used to check the design during compile time or run time.

If you want to generate asynchronous assertions, you would typically use the `\texttt{\$assertion\_off,}' `\texttt{\$assertion\_on},' `\texttt{\$assume},' `\texttt{\$cover},' or `\texttt{\$fell},' `\texttt{\$rose}' constructs.

However, without more context, it's hard to provide a more specific answer. If you could provide more information about the expected behavior or the conditions you want to check, I could give a more precise answer.

For example, if you want to ensure that `rdata\_sel\_q' is always valid (i.e., it's either `RD\_CSR,' `RD\_GPR,' `RD\_DBGA,' or `RD\_DBGS'), you could use an assertion like this:
\lstset{style=mystyle2}
\begin{lstlisting}[language=Verilog]
always @(*) begin
  $assert_on;
  assert (rdata_sel_q inside {RD_CSR, RD_GPR, RD_DBGA, RD_DBGS}) else $error("Invalid rdata_sel_q value");
end
\end{lstlisting}

\end{tcolorbox}
