# Supplementary material for: Enhancing Large Language Models for Hardware Verification: A Novel SystemVerilog Assertion Dataset
Source: arXiv:2503.08923 source file (2025-03-11)
Supplement: Supplementary file 19 [file LLama3_example_listing_ND.tex]

% \lstset{style=mystyle}
% \begin{lstlisting}[language=Verilog]
% Here is the SystemVerilog property that corresponds to the given code:

% `property lc_state_valid_q_posedge;
%   @(posedge clk_i) ($rose(!rst_ni) |-> lc_state_valid_q === 1'b0) |-> lc_state_valid_q === lc_state_valid_d;
% endproperty`

% This property states that when the clock edge occurs, if the reset signal is asserted (i.e., `!rst_ni` is true), then `lc_state_valid_q` should be 0. If the reset signal is not asserted, then `lc_state_valid_q` should be equal to `lc_state_valid_d`. 

% Note that the `rose` function is used to check if the reset signal is asserted (i.e., goes from 0 to 1) at the current clock edge.
% \end{lstlisting}

\begin{tcolorbox}[colback=white, colframe=black, boxrule=0.2mm, sharp corners, title=Llama 3.1 base model response, coltitle=black, colbacktitle=white]
Here is the list of synchronous SystemVerilog assertions that can be generated from the given code, executing at posedge HCLK:
\lstset{style=mystyle2}

\begin{lstlisting}[language=Verilog]
property p_reset_default_value;
    @(posedge HCLK) disable iff (~HRESETn) $rose(r_status) == 1;
endproperty
\end{lstlisting}

\begin{lstlisting}[language=Verilog]
property p_int_status_set;
    @(posedge HCLK) disable iff (~HRESETn) (s_rise_int) |=> (r_status | s_is_int_all);
endproperty
\end{lstlisting}

\begin{lstlisting}[language=Verilog]
property p_apb_reset_int_status;
    @(posedge HCLK) disable iff (~HRESETn) (PSEL && PENABLE &&!PWRITE && (s_apb_addr == `REG_INTSTATUS)) |=> (r_status == 'h0);
endproperty
\end{lstlisting}

Note: The `disable iff` keyword is used to disable the property when the condition is false. The `rose` function is used to check if the value of `r\_status` has risen (i.e., changed from 0 to 1) at the current clock edge. The `|=>` operator is used to specify the implication relationship between the antecedent and the consequent.

\end{tcolorbox}
